# Supplementary material for: Current-induced quasiparticle magnetic multipole moments
Source: arXiv:2210.15753 ancillary file (2022-10-27)
Supplement: Supplementary file 1 [file cim3_supp.pdf]

# Supplementary Information for "Current-induced quasiparticle magnetic multipole moments"

Muhammad Tahir[1] and Hua Chen[1,2]

[1] *Department of Physics, Colorado State University, Fort Collins, CO 80523, USA*
[2] *School of Advanced Materials Discovery, Colorado State University, Fort Collins, CO 80523, USA*

## I. GAUGE-INVARIANT FORMULA OF ARBITRARY-ORDER SPIN MAGNETIC MULTIPOLE MOMENTS OF A BLOCH WAVE PACKET

We start by considering non-degenerate bands and defining a wavepacket for the $n$-th band

$$|W\rangle = \int_{\rm BZ} d^3\mathbf{k} w_{\mathbf{k}} |n\mathbf{k}\rangle \tag{1}$$

where $|n\mathbf{k}\rangle$ is a Bloch state and $w_{\mathbf{k}}$ is a complex function localized about $\mathbf{k}_c$. We choose the normalization of Bloch functions as [1]

$$\langle n\mathbf{k}|m\mathbf{k}'\rangle = \frac{(2\pi)^3}{V_{\rm uc}}\delta_{nm}\delta(\mathbf{k}-\mathbf{k}'). \tag{2}$$

This is motivated by the fact that in the $N\to\infty$ limit there should be the relation

$$\delta_{\mathbf{k},\mathbf{k}'} \to \frac{(2\pi)^3}{V}\delta(\mathbf{k}-\mathbf{k}'). \tag{3}$$

which means

$$\begin{aligned}\langle u_{n\mathbf{k}}|u_{m\mathbf{k}'}\rangle &= \int d^3\mathbf{r} u^\dagger_{n\mathbf{k}} u_{m\mathbf{k}'} = N\int_{\rm uc} d^3\mathbf{r} u^\dagger_{n\mathbf{k}} u_{m\mathbf{k}'} \\ &= N\delta_{nm}\delta_{\mathbf{k},\mathbf{k}'} \to \frac{(2\pi)^3}{V_{\rm uc}}\delta_{nm}\delta(\mathbf{k}-\mathbf{k}').\end{aligned} \tag{4}$$

For later convenience, instead of Eq. (4) we define the inner product $\langle u_{n\mathbf{k}}|u_{m\mathbf{k}'}\rangle$ as

$$\langle u_{n\mathbf{k}}|u_{m\mathbf{k}'}\rangle \equiv \int_{\rm uc} d^3\mathbf{r} u^\dagger_{n\mathbf{k}} u_{m\mathbf{k}'} = \delta_{nm}\delta_{\mathbf{k},\mathbf{k}'} \to \frac{(2\pi)^3}{NV_{\rm uc}}\delta_{nm}\delta(\mathbf{k}-\mathbf{k}'). \tag{5}$$

Note that this means

$$\langle n\mathbf{k}|m\mathbf{k}'\rangle = \sum_{\mathbf{R}} e^{i(\mathbf{k}'-\mathbf{k})\cdot\mathbf{R}}\langle u_{n\mathbf{k}}|e^{i(\mathbf{k}'-\mathbf{k})\cdot\mathbf{R}}|u_{m\mathbf{k}'}\rangle = N\delta_{\mathbf{k},\mathbf{k}'}\langle u_{n\mathbf{k}}|u_{m\mathbf{k}}\rangle \to \frac{(2\pi)^3}{V_{\rm uc}}\delta_{nm}\delta(\mathbf{k}-\mathbf{k}'). \tag{6}$$

Namely, it is still consistent with Eq. (2). The benefit is that we do not have factors of $N$ when calculating the inner products among $|u_{n\mathbf{k}}\rangle$ or constructing the resolution of identity.

In addition, the Wannier functions, defined as

$$\begin{aligned}|n\mathbf{k}\rangle &= \sum_{\mathbf{R}} e^{i\mathbf{k}\cdot\mathbf{R}}|n\mathbf{R}\rangle, \\ |n\mathbf{R}\rangle &= \frac{V_{\rm uc}}{(2\pi)^3}\int_{\rm BZ} d^3\mathbf{k} e^{-i\mathbf{k}\cdot\mathbf{R}}|n\mathbf{k}\rangle\end{aligned} \tag{7}$$

is normalized as

$$\langle n\mathbf{R}|m\mathbf{R}'\rangle = \delta_{nm}\delta_{\mathbf{R},\mathbf{R}'}. \tag{8}$$

We then have the resolution of identity:

$$\begin{aligned}\mathbb{I} &= \frac{V_{\rm uc}}{(2\pi)^3}\sum_n\int_{\rm BZ} d^3\mathbf{k}|n\mathbf{k}\rangle\langle n\mathbf{k}| = \frac{NV_{\rm uc}}{(2\pi)^3}\sum_n\int_{\rm BZ} d^3\mathbf{k}|u_{n\mathbf{k}}\rangle\langle u_{n\mathbf{k}}| \\ &= \frac{1}{N}\sum_{n\mathbf{k}}|n\mathbf{k}\rangle\langle n\mathbf{k}| = \sum_{n\mathbf{k}}|u_{n\mathbf{k}}\rangle\langle u_{n\mathbf{k}}|\end{aligned} \tag{9}$$

Eq. (2) and $\langle W|W\rangle = 1$ together lead to

$$\int_{\mathrm{BZ}} d^3\mathbf{k}|w_\mathbf{k}|^2 = \frac{V_{\mathrm{uc}}}{(2\pi)^3}. \tag{10}$$

The center of mass of $|W\rangle$ is

$$\langle W|\mathbf{r}|W\rangle \equiv \mathbf{r}_c. \tag{11}$$

$\mathbf{r}_c$ can be calculated more explicitly:

$$\mathbf{r}_c = \int_{\mathrm{BZ}} d^3\mathbf{k}d^3\mathbf{k}' w^*_\mathbf{k} w_{\mathbf{k}'} \langle n\mathbf{k}|\mathbf{r}|n\mathbf{k}'\rangle \tag{12}$$

The matrix elements of $\mathbf{r}$ in Bloch state representation are

$$\langle n\mathbf{k}|\mathbf{r}|m\mathbf{k}'\rangle = -i\delta_{nm}\partial_{\mathbf{k}'}\delta(\mathbf{k}-\mathbf{k}')\frac{(2\pi)^3}{V_{\mathrm{uc}}} + \frac{(2\pi)^3}{V_{\mathrm{uc}}}\delta(\mathbf{k}'-\mathbf{k})\langle u_{n\mathbf{k}}|i\partial_\mathbf{k}|u_{m\mathbf{k}}\rangle \tag{13}$$

As a result

$$\mathbf{r}_c = \frac{(2\pi)^3}{V_{\mathrm{uc}}}\int_{\mathrm{BZ}} d^3\mathbf{k}\left[i(w^*_\mathbf{k}\partial_\mathbf{k} w_\mathbf{k}) + \langle u_{n\mathbf{k}}|i\partial_\mathbf{k}|u_{n\mathbf{k}}\rangle |w_\mathbf{k}|^2\right]. \tag{14}$$

When the wavepacket is localized in the momentum space, we have

$$\begin{aligned}\mathbf{r}_c &\approx \frac{(2\pi)^3}{V_{\mathrm{uc}}}\int_{\mathrm{BZ}} d^3\mathbf{k}|w_\mathbf{k}|^2\left[\frac{i(w^*_\mathbf{k}\partial_\mathbf{k} w_\mathbf{k})}{|w_\mathbf{k}|^2} + \langle u_{n\mathbf{k}}|i\partial_\mathbf{k}|u_{n\mathbf{k}}\rangle\right]_{\mathbf{k}=\mathbf{k}_c} \\ &= \left[\frac{i(w^*_\mathbf{k}\partial_\mathbf{k} w_\mathbf{k})}{|w_\mathbf{k}|^2} + \langle u_{n\mathbf{k}}|i\partial_\mathbf{k}|u_{n\mathbf{k}}\rangle\right]_{\mathbf{k}=\mathbf{k}_c}.\end{aligned} \tag{15}$$

For real wavepackets the first term vanishes. However, the second term is gauge dependent, indicating that the center-of-mass position of a Bloch wavepacket does not have a definite value.

The motivation of subtracting $\mathbf{r}_c$ from $\mathbf{r}$ in the definition of the wavepacket magnetic multipole moments is to eliminate the gauge dependence from a naive definition of the multipole moment:

$$\begin{aligned}(\mathcal{M}^g)^{i_l}_{i_1 i_2 \ldots i_{l-1}} &\equiv \langle W|\prod_{n=1}^{l-1}(\mathbf{r})_{i_n} s_{i_l}|W\rangle \\ &= \langle W|x^{N_x}y^{N_y}z^{N_z}s_{i_l}|W\rangle\end{aligned} \tag{16}$$

where the last equality is due to the fact that position operators commute with one another; $N_x + N_y + N_z = l-1$. However, we will see below that such a naive approach does not warrant gauge invariance. Alternatively, we can directly perform a gauge transformation in $\mathcal{M}^g$ and see how the terms it produces can be removed.

For convenience we use the position representation. Eq. (16) becomes

$$\begin{aligned}\mathcal{M}^g &= \int d^3\mathbf{k}\int d^3\mathbf{k}' w^*_\mathbf{k} w_{\mathbf{k}'}\langle n\mathbf{k}|x^{N_x}y^{N_y}z^{N_z}\mathbf{s}|n\mathbf{k}'\rangle \\ &= \int d^3\mathbf{k}\int d^3\mathbf{k}'\int d^3\mathbf{r} e^{i(\mathbf{k}'-\mathbf{k})\cdot\mathbf{r}} w^*_\mathbf{k} u^\dagger_{n\mathbf{k}}\mathbf{s}\left[(i\partial_{k'_x})^{N_x}(i\partial_{k'_y})^{N_y}(i\partial_{k'_z})^{N_z}(w_{\mathbf{k}'}u_{n\mathbf{k}'})\right] \\ &= \int d^3\mathbf{k}\int d^3\mathbf{k}'\sum_\mathbf{R} e^{i(\mathbf{k}'-\mathbf{k})\cdot\mathbf{R}}\int_{\mathrm{uc}} d^3\mathbf{r} e^{i(\mathbf{k}'-\mathbf{k})\cdot\mathbf{r}} w^*_\mathbf{k} u^\dagger_{n\mathbf{k}}\mathbf{s}\left[(i\partial_{k'_x})^{N_x}(i\partial_{k'_y})^{N_y}(i\partial_{k'_z})^{N_z}(w_{\mathbf{k}'}u_{n\mathbf{k}'})\right] \\ &= \frac{(2\pi)^3}{V_{\mathrm{uc}}}\int_{\mathbf{k},\mathbf{k}'}\sum_\mathbf{G}\delta(\mathbf{k}'-\mathbf{k}-\mathbf{G})\int_{\mathrm{uc}} d^3\mathbf{r} e^{i(\mathbf{k}'-\mathbf{k})\cdot\mathbf{r}} w^*_\mathbf{k} u^\dagger_{n\mathbf{k}}\mathbf{s}\left[(i\partial_{k'_x})^{N_x}(i\partial_{k'_y})^{N_y}(i\partial_{k'_z})^{N_z}(w_{\mathbf{k}'}u_{n\mathbf{k}'})\right] \\ &= \frac{(2\pi)^3}{V_{\mathrm{uc}}}\int d^3\mathbf{k} w^*_\mathbf{k}\langle u_{n\mathbf{k}}|\mathbf{s}(i\partial_{k_x})^{N_x}(i\partial_{k_y})^{N_y}(i\partial_{k_z})^{N_z}(w_\mathbf{k}|u_{n\mathbf{k}}\rangle).\end{aligned} \tag{17}$$

We now perform an arbitrary gauge transformation

$$u_{n\mathbf{k}}(\mathbf{r}) \to e^{i\phi(\mathbf{k})} u_{n\mathbf{k}}(\mathbf{r}). \tag{18}$$

To see what such a transformation leads to, note that in general

$$(\partial_x)^n e^{f(x)} = e^{f(x)} B_n \left(f', f'', \ldots, f^{(n)}\right) \tag{19}$$

where $B_n$ is the $n$-th order Bell polynomial. Therefore

$$e^{-i\phi}(\partial_x)^{i_x}(\partial_y)^{i_y}(\partial_z)^{i_z} e^{i\phi} = e^{-i\phi}(\partial_x)^{i_x}(\partial_y)^{i_y}\left[e^{i\phi} B_{i_z}[i\partial_z\phi]\right] \equiv \mathcal{F}_{i_x,i_y,i_z}[\nabla\phi] \tag{20}$$

where $\mathcal{F}$ is a complicated functional of the gradient of $\phi$, involving polynomials of higher-order derivatives of $\nabla\phi$. Therefore such terms in general cannot be removed by a simple replacement of $\mathbf{r}$ by $\mathbf{r} - \mathbf{r}_c$ in the definition of $\mathcal{M}^g$. Instead, we use Eq. (4) in the main text which leads to the following conclusion:

$$\langle u_{n\mathbf{k}}|\mathbf{s}\left(i\partial_{k_j} - \langle u_{n\mathbf{k}}|i\partial_{k_j}|u_{n\mathbf{k}}\rangle\right)^{N_j}|u_{n\mathbf{k}}\rangle \tag{21}$$

is gauge invariant. To see how this equation can be connected with $\mathcal{M}^g$ in Eq. (17), we consider

$$\begin{aligned} \mathcal{M}^g &= \langle W|x^{N_x}\mathbf{s}|W\rangle \\ &= \frac{(2\pi)^3}{V_{\text{uc}}}\int d^3\mathbf{k} w^*_{\mathbf{k}}\langle u_{n\mathbf{k}}|\mathbf{s}\left[(i\partial_{k_x})^{N_x} w_{\mathbf{k}}|u_{n\mathbf{k}}\rangle\right] \end{aligned} \tag{22}$$

The identity of Eq. (4) in the main text leads to a gauge invariant counterpart of $\mathcal{M}^g$:

$$\begin{aligned} \mathcal{M} &\equiv \frac{(2\pi)^3}{V_{\text{uc}}}\text{Re}\int d^3\mathbf{k} w^*_{\mathbf{k}}\langle u_{n\mathbf{k}}|\mathbf{s}\left[(i\partial_{k_x} - \mathcal{A}_x - i\partial_{k_x}\ln|w_{\mathbf{k}}| + \partial_{k_x}\arg w_{\mathbf{k}})^{N_x} w_{\mathbf{k}}|u_{n\mathbf{k}}\rangle\right] \\ &= \frac{(2\pi)^3}{V_{\text{uc}}}\text{Re}\int d^3\mathbf{k}|w_{\mathbf{k}}|^2\langle u_{n\mathbf{k}}|\mathbf{s}(i\partial_{k_x} - \mathcal{A}_x)^{N_x}|u_{n\mathbf{k}}\rangle \\ &\approx \text{Re}\langle u_{n\mathbf{k}}|\mathbf{s}(i\partial_{k_x} - \mathcal{A}_x)^{N_x}|u_{n\mathbf{k}}\rangle\big|_{\mathbf{k}=\mathbf{k}_c} \end{aligned} \tag{23}$$

where $\mathcal{A}_x \equiv \langle u_{n\mathbf{k}}|i\partial_{k_x}|u_{n\mathbf{k}}\rangle$. Eq. (23) can be viewed as a more concrete version of the naive construction:

$$\mathcal{M}^{i_l}_{i_1 i_2 \ldots i_{l-1}} \equiv \langle W|\prod_{n=1}^{l-1}(\mathbf{r} - \mathbf{r}_c)_{i_n} s_{i_l}|W\rangle \tag{24}$$

which is not only dependent on the wave packet shape but is also not necessarily gauge invariant. This can be seen by considering $\mathcal{M}^x_{xxx}$:

$$\begin{aligned} \mathcal{M}^x_{xxx} &= \langle W|(x - x_c)^3 s_x|W\rangle = \langle W|x^3 s_x|W\rangle - 3x_c\langle W|x^2 s_x|W\rangle + 3x_c^2\langle W|x s_x|W\rangle - x_c^3\langle W|s_x|W\rangle \\ &\to \langle u_{n\mathbf{k}_c}|s_x(i\partial_{k_{cx}})^3|u_{n\mathbf{k}_c}\rangle - 3x_c\langle u_{n\mathbf{k}_c}|(i\partial_{k_{cx}})^2 s_x|u_{n\mathbf{k}_c}\rangle + 3x_c^2\langle u_{n\mathbf{k}_c}|(i\partial_{k_{cx}})s_x|u_{n\mathbf{k}_c}\rangle - x_c^3\langle u_{n\mathbf{k}_c}|s_x|u_{n\mathbf{k}_c}\rangle \\ &= \langle u_{n\mathbf{k}_c}|s_x(i\partial_{k_{cx}} - x_c)^3|u_{n\mathbf{k}_c}\rangle \\ &- \left\{-3(i\partial_{k_x}x_c)\langle u_{n\mathbf{k}_c}|(i\partial_{k_{cx}})s_x|u_{n\mathbf{k}_c}\rangle + (\partial^2_{k_x}x_c)\langle u_{n\mathbf{k}_c}|s_x|u_{n\mathbf{k}_c}\rangle + 3x_c(i\partial_{k_x}x_c)\langle u_{n\mathbf{k}_c}|s_x|u_{n\mathbf{k}_c}\rangle\right\} \end{aligned} \tag{25}$$

The terms in the curly brackets are in general nonzero. Even if the first and last term are dropped since they are imaginary, the second term is in general real and gauge dependent. One can also understand why the case of octupole moment is not a concern, since the difference between Eq. (24) and Eq. (23) is purely imaginary (see below).

We next consider the case when there are mixed spatial components $\mathcal{M}^g$. In this case $i\partial_{k_x} - \mathcal{A}_x$ does not commute with $i\partial_{k_y} - \mathcal{A}_y$. Specifically, we would like to prove first

$$\prod_{\{x_j\}_n}(i\partial_{x_j} - A_{x_j} - i\partial_{x_j}\ln|g| + \partial_{x_j}\arg g)(gf) = g\prod_{\{x_j\}_n}(i\partial_{x_j} - A_{x_j})f \tag{26}$$

where $x_j$ is the $j$'s element of an arbitrary sequence of length $n$, $\{x_j\}_n \equiv \{x, z, y, x, \ldots\}$, with Cartesian indices as its elements. Eq. (26) can be straightforwardly proved by induction similar to Eq. (4) in the main text. Then we define the general $\mathcal{M}$ as

$$\mathcal{M} \equiv \mathcal{N}^{-1}\text{Re}\sum_{\{j\}^{\text{u}}_{l-1}}\langle u_{n\mathbf{k}}|\mathbf{s}\prod_{j\in\{j\}^{\text{u}}_{l-1}}(i\partial_{k_j} - \mathcal{A}_j)|u_{n\mathbf{k}}\rangle\big|_{\mathbf{k}=\mathbf{k}_c} \tag{27}$$

where the summation is over all non-repeating sequences of $l-1$ elements, in which the Cartesian index $j$ appears exactly $N_j$ times. The normalization factor $\mathcal{N} = (l-1)!/(N_x!N_y!N_z!)$. The summation over $\{j\}^{\mathrm{u}}_{l-1}$ ensures that $\mathcal{M}^{\bar{w}}$ is always invariant under arbitrary permutations of its spatial components, which is a property of the gauge-dependent form $\mathcal{M}^g$ that must be carried over.

As an application of Eq. (27), we consider the mixed octupole moment $\mathcal{M}^z_{xy}$, where $z$ is the spin component:

$$\begin{aligned} \mathcal{M}^z_{xy} &= \frac{1}{2}\mathrm{Re}\langle u_{n\mathbf{k}}|s_z\left[(i\partial_{k_x}-\mathcal{A}_x),(i\partial_{k_y}-\mathcal{A}_y)\right]_+|u_{n\mathbf{k}}\rangle\big|_{\mathbf{k}=\mathbf{k}_c} \\ &= -\langle s_z\partial_{k_x}\partial_{k_y}\rangle + \mathcal{A}_x\mathcal{A}_y\langle s_z\rangle - \mathcal{A}_x\langle is_z\partial_{k_y}\rangle - \mathcal{A}_y\langle is_z\partial_{k_x}\rangle. \end{aligned} \tag{28}$$

Since $\mathcal{M}^z_{xy}$ is gauge invariant we can use any gauge to calculate it. We will choose $\mathcal{A}=0$, which however does not imply that the derivatives of $\mathcal{A}$ are zero. Fortunately, since $\mathcal{A}$ is real, such derivatives only appear in a purely imaginary term and is omitted in the above equation. The final result is

$$\mathcal{M}^z_{xy} = -\langle s_z\partial_{k_x}\partial_{k_y}\rangle\big|_{\mathcal{A}=0} \tag{29}$$

To write the above result in terms of matrix elements of known quantities, such as those of the spin operator and $k$-derivatives of the Hamiltonian, we need to evaluate the derivative of the Bloch states using perturbation theory, which will be done in the next section.

## II. EXPLICIT FORMULAS OF THE SPIN OCTUPOLE AND HEXADECAPOLE MOMENTS OF A BLOCH WAVE PACKET

In this section we give explicit formulas of some low-order magnetic multipole moments. Our main goal is the hexadecapole ($l=4$), which requires the third order $k$-derivative of $|u_{n\mathbf{k}}\rangle$. Since in previous literature only the first-order derivative formula is given, below we first give the third order derivative using perturbation theory. We start from the eigenequation

$$H_{\mathbf{k}}|u_{n\mathbf{k}}\rangle = \epsilon_{n\mathbf{k}}|u_{n\mathbf{k}}\rangle \tag{30}$$

and consider the equation at $\mathbf{k}+\delta\mathbf{k}$, where $\delta\mathbf{k}$ is small:

$$H_{\mathbf{k}+\delta\mathbf{k}}|u_{n\mathbf{k}+\delta\mathbf{k}}\rangle = \epsilon_{n\mathbf{k}+\delta\mathbf{k}}|u_{n\mathbf{k}+\delta\mathbf{k}}\rangle. \tag{31}$$

$H_{\mathbf{k}+\delta\mathbf{k}}$, $|u_{n\mathbf{k}+\delta\mathbf{k}}\rangle$, and $\epsilon_{n\mathbf{k}+\delta\mathbf{k}}$ can be Taylor expanded as (up to 2nd order; the 3rd order result will be given separately below)

$$\begin{aligned} H_{\mathbf{k}+\delta\mathbf{k}} &\approx H_{\mathbf{k}} + \partial_a H_{\mathbf{k}}\delta k_a + \frac{1}{2}\partial_a\partial_b H_{\mathbf{k}}\delta k_a\delta k_b \\ |u_{n\mathbf{k}+\delta\mathbf{k}}\rangle &\approx |u_{n\mathbf{k}}\rangle + \partial_a|u_{n\mathbf{k}}\rangle\delta k_a + \frac{1}{2}\partial_a\partial_b|u_{n\mathbf{k}}\rangle\delta k_a\delta k_b \\ \epsilon_{n\mathbf{k}+\delta\mathbf{k}} &\approx \epsilon_{n\mathbf{k}} + \partial_a\epsilon_{n\mathbf{k}}\delta k_a + \frac{1}{2}\partial_a\partial_b\epsilon_{n\mathbf{k}}\delta k_a\delta k_b \end{aligned} \tag{32}$$

Note that the derivatives of $\epsilon_{n\mathbf{k}}$ should also be understood as unknown variables to be solved from the perturbation equations. Substituting Eq. (32) into Eq. (31) gives the following equations at increasing powers of $\delta k$:

$$\begin{aligned} &H_{\mathbf{k}}|u_{n\mathbf{k}}\rangle = \epsilon_{n\mathbf{k}}|u_{n\mathbf{k}}\rangle \\ &\partial_a H_{\mathbf{k}}|u_{n\mathbf{k}}\rangle + H_{\mathbf{k}}\partial_a|u_{n\mathbf{k}}\rangle = \epsilon_{n\mathbf{k}}\partial_a|u_{n\mathbf{k}}\rangle + \partial_a\epsilon_{n\mathbf{k}}|u_{n\mathbf{k}}\rangle \\ &\big(\partial_a\partial_b H_{\mathbf{k}}|u_{n\mathbf{k}}\rangle + \partial_a H_{\mathbf{k}}\partial_b|u_{n\mathbf{k}}\rangle + \partial_b H_{\mathbf{k}}\partial_a|u_{n\mathbf{k}}\rangle + H_{\mathbf{k}}\partial_a\partial_b|u_{n\mathbf{k}}\rangle\big) \\ &= \big(\epsilon_{n\mathbf{k}}\partial_a\partial_b|u_{n\mathbf{k}}\rangle + \partial_a\epsilon_{n\mathbf{k}}\partial_b|u_{n\mathbf{k}}\rangle + \partial_b\epsilon_{n\mathbf{k}}\partial_a|u_{n\mathbf{k}}\rangle + \partial_a\partial_b\epsilon_{n\mathbf{k}}|u_{n\mathbf{k}}\rangle\big) \end{aligned} \tag{33}$$

In addition, the normalization condition $\langle u_{n\mathbf{k}+\delta\mathbf{k}}|u_{n\mathbf{k}+\delta\mathbf{k}}\rangle = 1$ leads to the following equations, also at increasing powers of $\delta k$:

$$\begin{aligned} &\langle u_{n\mathbf{k}}|u_{n\mathbf{k}}\rangle = 1 \\ &\mathrm{Re}\langle u_{n\mathbf{k}}|\partial_a|u_{n\mathbf{k}}\rangle = 0 \\ &\mathrm{Re}\langle u_{n\mathbf{k}}|\partial_a\partial_b|u_{n\mathbf{k}}\rangle + \mathrm{Re}\langle\partial_a u_{n\mathbf{k}}|\partial_b u_{n\mathbf{k}}\rangle = 0 \end{aligned} \tag{34}$$

Since $\sum_n |u_{n\mathbf{k}}\rangle\langle u_{n\mathbf{k}}| = \mathbb{I}$, we have in general

$$\begin{aligned}\partial_a|u_{n\mathbf{k}}\rangle &= \langle u_{n\mathbf{k}}|\partial_a|u_{n\mathbf{k}}\rangle|u_{n\mathbf{k}}\rangle + \sum_{m\neq n}\langle u_{m\mathbf{k}}|\partial_a|u_{n\mathbf{k}}\rangle|u_{m\mathbf{k}}\rangle \\ \partial_a\partial_b|u_{n\mathbf{k}}\rangle &= \langle u_{n\mathbf{k}}|\partial_a\partial_b|u_{n\mathbf{k}}\rangle|u_{n\mathbf{k}}\rangle + \sum_{m\neq n}\langle u_{m\mathbf{k}}|\partial_a\partial_b|u_{n\mathbf{k}}\rangle|u_{m\mathbf{k}}\rangle\end{aligned} \tag{35}$$

However, the first term in each equation cannot be obtained from the eigenequations Eq. (33) alone, since multiplying the eigenequation from the left by $\langle u_{n\mathbf{k}}|$ just gives identities. Therefore the normalization condition Eq. (34) is necessary.

We now multiply $\langle u_{m\mathbf{k}}|$, $m \neq n$, from the left to the 1st and 2nd order eigenequations. The first order equation becomes

$$(\partial_a H_{\mathbf{k}})_{mn} + \langle u_{m\mathbf{k}}|\partial_a|u_{n\mathbf{k}}\rangle\epsilon_{m\mathbf{k}} = \epsilon_{n\mathbf{k}}\langle u_{m\mathbf{k}}|\partial_a|u_{n\mathbf{k}}\rangle \tag{36}$$

which leads to (we do not consider the case of degenerate levels, i.e. $\epsilon_{n\mathbf{k}} \neq \epsilon_{m\mathbf{k}}$)

$$\langle u_{m\mathbf{k}}|\partial_a|u_{n\mathbf{k}}\rangle = \frac{(\partial_a H_{\mathbf{k}})_{mn}}{\epsilon_{n\mathbf{k}} - \epsilon_{m\mathbf{k}}}. \tag{37}$$

Namely, we have all coefficients in the second term of Eq. (35) for $\partial_a|u_{n\mathbf{k}}\rangle$. The first term, however, requires the second equation in Eq. (34). Since $\langle u_{n\mathbf{k}}|\partial_a|u_{n\mathbf{k}}\rangle$ is purely imaginary, we can define $\langle u_{n\mathbf{k}}|\partial_a|u_{n\mathbf{k}}\rangle \equiv -i\mathcal{A}_a$ where the Berry connection $\mathcal{A}_a$ is real. As a result

$$\partial_a|u_{n\mathbf{k}}\rangle = -i\mathcal{A}_a|u_{n\mathbf{k}}\rangle + \sum_{m\neq n}\frac{(\partial_a H_{\mathbf{k}})_{mn}}{\epsilon_{n\mathbf{k}} - \epsilon_{m\mathbf{k}}}|u_{m\mathbf{k}}\rangle. \tag{38}$$

The usual formula with only the second term in the above equation therefore corresponds to a gauge choice of $\mathcal{A} = 0$.

Similarly, the second order eigenequation becomes

$$\begin{aligned}&(\partial_a\partial_b H_{\mathbf{k}})_{mn} + \langle u_{m\mathbf{k}}|(\partial_a H_{\mathbf{k}})|\partial_b u_{n\mathbf{k}}\rangle + \langle u_{m\mathbf{k}}|(\partial_b H_{\mathbf{k}})|\partial_a u_{n\mathbf{k}}\rangle + \epsilon_{m\mathbf{k}}\langle u_{m\mathbf{k}}|\partial_a\partial_b|u_{n\mathbf{k}}\rangle \\ &= \epsilon_{n\mathbf{k}}\langle u_{m\mathbf{k}}|\partial_a\partial_b|u_{n\mathbf{k}}\rangle + \partial_a\epsilon_{n\mathbf{k}}\langle u_{m\mathbf{k}}|\partial_b|u_{n\mathbf{k}}\rangle + \partial_b\epsilon_{n\mathbf{k}}\langle u_{m\mathbf{k}}|\partial_a|u_{n\mathbf{k}}\rangle\end{aligned} \tag{39}$$

which simplifies to

$$\langle u_{m\mathbf{k}}|\partial_a\partial_b|u_{n\mathbf{k}}\rangle = \frac{(\partial_a\partial_b H_{\mathbf{k}})_{mn} + \langle u_{m\mathbf{k}}|\partial_a(H_{\mathbf{k}} - \epsilon_{n\mathbf{k}})|\partial_b u_{n\mathbf{k}}\rangle + \langle u_{m\mathbf{k}}|\partial_b(H_{\mathbf{k}} - \epsilon_{n\mathbf{k}})|\partial_a u_{n\mathbf{k}}\rangle}{\epsilon_{n\mathbf{k}} - \epsilon_{m\mathbf{k}}}. \tag{40}$$

To go further, we can substitute Eq. (38) into the second and third terms in the denominator of the above equation, which leads to

$$\langle u_{m\mathbf{k}}|\partial_a(H_{\mathbf{k}} - \epsilon_{n\mathbf{k}})|\partial_b u_{n\mathbf{k}}\rangle = -i\mathcal{A}_b(\partial_a H_{\mathbf{k}})_{mn} + \sum_{l\neq n}\frac{(\partial_b H_{\mathbf{k}})_{ln}\left[(\partial_a H_{\mathbf{k}})_{ml} - (\partial_a H_{\mathbf{k}})_{nn}\delta_{ml}\right]}{\epsilon_{n\mathbf{k}} - \epsilon_{l\mathbf{k}}} \tag{41}$$

As a result

$$\langle u_{m\mathbf{k}}|\partial_a\partial_b|u_{n\mathbf{k}}\rangle = \frac{(\partial_a\partial_b H_{\mathbf{k}})_{mn}}{\epsilon_{n\mathbf{k}} - \epsilon_{m\mathbf{k}}} + \left\{-i\mathcal{A}_b\frac{(\partial_a H_{\mathbf{k}})_{mn}}{\epsilon_{n\mathbf{k}} - \epsilon_{m\mathbf{k}}} + \sum_{l\neq n}\frac{(\partial_b H_{\mathbf{k}})_{ln}\left[(\partial_a H_{\mathbf{k}})_{ml} - (\partial_a H_{\mathbf{k}})_{nn}\delta_{ml}\right]}{(\epsilon_{n\mathbf{k}} - \epsilon_{l\mathbf{k}})(\epsilon_{n\mathbf{k}} - \epsilon_{m\mathbf{k}})} + (a \leftrightarrow b)\right\} \tag{42}$$

which gives all coefficients in the second term of the second equation in Eq. (35). The first term must be determined by the last equation in Eq. (34). The real part of $\langle u_{n\mathbf{k}}|\partial_a\partial_b|u_{n\mathbf{k}}\rangle$ is equal to

$$\begin{aligned}\mathrm{Re}\langle u_{n\mathbf{k}}|\partial_a\partial_b|u_{n\mathbf{k}}\rangle &= -\mathrm{Re}\langle\partial_a u_{n\mathbf{k}}|\partial_b u_{n\mathbf{k}}\rangle \\ &= \mathrm{Re}\left\{\langle u_{n\mathbf{k}}|\partial_a|u_{n\mathbf{k}}\rangle\langle u_{n\mathbf{k}}|\partial_b|u_{n\mathbf{k}}\rangle + \sum_{m\neq n}\langle u_{n\mathbf{k}}|\partial_a|u_{m\mathbf{k}}\rangle\langle u_{m\mathbf{k}}|\partial_b|u_{n\mathbf{k}}\rangle\right\} \\ &= -\mathcal{A}_a\mathcal{A}_b - \mathrm{Re}\sum_{m\neq n}\frac{(\partial_a H_{\mathbf{k}})_{nm}(\partial_b H_{\mathbf{k}})_{mn}}{(\epsilon_{n\mathbf{k}} - \epsilon_{m\mathbf{k}})^2}\end{aligned} \tag{43}$$

The imaginary part of $\langle u_{n\mathbf{k}}|\partial_a\partial_b|u_{n\mathbf{k}}\rangle$ is, however, undetermined. Note that

$$\begin{aligned}\mathrm{Im}\langle u_{n\mathbf{k}}|\partial_a\partial_b|u_{n\mathbf{k}}\rangle &= \mathrm{Im}\partial_a\langle u_{n\mathbf{k}}|\partial_b|u_{n\mathbf{k}}\rangle - \mathrm{Im}\langle\partial_a u_{n\mathbf{k}}|\partial_b u_{n\mathbf{k}}\rangle \\ &= -\partial_a\mathcal{A}_b - \mathrm{Im}\sum_{m\neq n}\frac{(\partial_a H_{\mathbf{k}})_{nm}(\partial_b H_{\mathbf{k}})_{mn}}{(\epsilon_{n\mathbf{k}}-\epsilon_{m\mathbf{k}})^2}\end{aligned} \tag{44}$$

Taken together,

$$\langle u_{n\mathbf{k}}|\partial_a\partial_b|u_{n\mathbf{k}}\rangle = -\mathcal{A}_a\mathcal{A}_b - i\partial_a\mathcal{A}_b - \sum_{m\neq n}\frac{(\partial_a H_{\mathbf{k}})_{nm}(\partial_b H_{\mathbf{k}})_{mn}}{(\epsilon_{n\mathbf{k}}-\epsilon_{m\mathbf{k}})^2} \tag{45}$$

Eqs. 42 and 45 then give the 2nd order derivative of $|u_{n\mathbf{k}}\rangle$ through Eq. (35).

We now turn to the 3rd order derivative. The 3rd order counterparts of Eqs. (33) and (34) are

$$\begin{aligned}&(H_{\mathbf{k}}-\epsilon_{n\mathbf{k}})|\partial_a\partial_b\partial_c u_{n\mathbf{k}}\rangle + \partial_a\partial_b\partial_c(H_{\mathbf{k}}-\epsilon_{n\mathbf{k}})|u_{n\mathbf{k}}\rangle \\ &+[\partial_a(H_{\mathbf{k}}-\epsilon_{n\mathbf{k}})|\partial_b\partial_c u_{n\mathbf{k}}\rangle + (b,ca)+(c,ab)] + [\partial_a\partial_b(H_{\mathbf{k}}-\epsilon_{n\mathbf{k}})|\partial_c u_{n\mathbf{k}}\rangle + (bc,a)+(ca,b)] = 0, \\ &\mathrm{Re}\langle u_{n\mathbf{k}}|\partial_a\partial_b\partial_c u_{n\mathbf{k}}\rangle + [\mathrm{Re}\langle\partial_a u_{n\mathbf{k}}|\partial_b\partial_c u_{n\mathbf{k}}\rangle + (b,ca)+(c,ab)] = 0\end{aligned} \tag{46}$$

Similar as before from the eigenequation we can obtain the inter-band matrix element with $m \neq n$:

$$\begin{aligned}&\langle u_{m\mathbf{k}}|\partial_a\partial_b\partial_c u_{n\mathbf{k}}\rangle = \frac{1}{\epsilon_{n\mathbf{k}}-\epsilon_{m\mathbf{k}}}\times\Big\{\langle u_{m\mathbf{k}}|\partial_a\partial_b\partial_c H_{\mathbf{k}}|u_{n\mathbf{k}}\rangle \\ &+[\langle u_{m\mathbf{k}}|\partial_a(H_{\mathbf{k}}-\epsilon_{n\mathbf{k}})|\partial_b\partial_c u_{n\mathbf{k}}\rangle + (b,ca)+(c,ab)] + [\langle u_{m\mathbf{k}}|\partial_a\partial_b(H_{\mathbf{k}}-\epsilon_{n\mathbf{k}})|\partial_c u_{n\mathbf{k}}\rangle + (bc,a)+(ca,b)]\Big\}\end{aligned} \tag{47}$$

since we have already obtained explicit results of the 1st and 2nd order derivatives of $|u_{n\mathbf{k}}\rangle$, the only unknown quantity in the above equation is $\partial_a\partial_b\epsilon_{n\mathbf{k}}$, which according to Eq. (33) is

$$\partial_a\partial_b\epsilon_{n\mathbf{k}} = \langle u_{n\mathbf{k}}|\partial_a\partial_b H_{\mathbf{k}}|u_{n\mathbf{k}}\rangle + \langle u_{n\mathbf{k}}|\partial_a(H_{\mathbf{k}}-\epsilon_{n\mathbf{k}})|\partial_b u_{n\mathbf{k}}\rangle + \langle u_{n\mathbf{k}}|\partial_b(H_{\mathbf{k}}-\epsilon_{n\mathbf{k}})|\partial_a u_{n\mathbf{k}}\rangle. \tag{48}$$

The real part of the intra-band matrix element can be obtained from the second equation of Eq. (46):

$$\mathrm{Re}\langle u_{n\mathbf{k}}|\partial_a\partial_b\partial_c u_{n\mathbf{k}}\rangle = -\mathrm{Re}\left[\langle\partial_a u_{n\mathbf{k}}|\partial_b\partial_c u_{n\mathbf{k}}\rangle + (b,ca)+(c,ab)\right], \tag{49}$$

while the imaginary part can be obtained as

$$\mathrm{Im}\langle u_{n\mathbf{k}}|\partial_a\partial_b\partial_c u_{n\mathbf{k}}\rangle = \mathrm{Im}\left[\partial_a\partial_b\langle u_{n\mathbf{k}}|\partial_c u_{n\mathbf{k}}\rangle + \langle\partial_c u_{n\mathbf{k}}|\partial_a\partial_b u_{n\mathbf{k}}\rangle - \langle\partial_a u_{n\mathbf{k}}|\partial_b\partial_c u_{n\mathbf{k}}\rangle - \langle\partial_b u_{n\mathbf{k}}|\partial_a\partial_c u_{n\mathbf{k}}\rangle\right]. \tag{50}$$

Taken together:

$$\begin{aligned}\langle u_{n\mathbf{k}}|\partial_a\partial_b\partial_c u_{n\mathbf{k}}\rangle &= -i\partial_a\partial_b\mathcal{A}_c + 2i\mathrm{Im}\langle\partial_c u_{n\mathbf{k}}|\partial_a\partial_b u_{n\mathbf{k}}\rangle - [\langle\partial_a u_{n\mathbf{k}}|\partial_b\partial_c u_{n\mathbf{k}}\rangle + (b,ca)+(c,ab)] \\ &= -i\partial_a\partial_b\mathcal{A}_c - [\langle\partial_a u_{n\mathbf{k}}|\partial_b\partial_c u_{n\mathbf{k}}\rangle + (b,ca)+(ab,c)]\end{aligned} \tag{51}$$

where the last equality is because $\langle\partial_a\partial_b u_{n\mathbf{k}}|\partial_c u_{n\mathbf{k}}\rangle = \langle\partial_c u_{n\mathbf{k}}|\partial_a\partial_b u_{n\mathbf{k}}\rangle^* = \langle\partial_c u_{n\mathbf{k}}|\partial_a\partial_b u_{n\mathbf{k}}\rangle - 2i\mathrm{Im}\langle\partial_c u_{n\mathbf{k}}|\partial_a\partial_b u_{n\mathbf{k}}\rangle$.

Eqs. (47), (48), and (51) together with the lower-order formulas Eqs. (42), (45), (38) give the full 3rd order derivative formula.

To apply our formulas we first use them to calculate the spin quadrupole moment and compare it with existing results in literature. The gauge-invariant spin quadrupole moment of the wave packet is

$$\mathcal{M}_a^b = \langle u_{n\mathbf{k}}|s_b(i\partial_a - \mathcal{A}_a)|u_{n\mathbf{k}}\rangle = i\langle u_{n\mathbf{k}}|s_b|\partial_a u_{n\mathbf{k}}\rangle - \mathcal{A}_a(s_b)_{nn} \tag{52}$$

Substituting Eq. (38) into the above equation, we obtain

$$\mathcal{M}_a^b = \mathcal{A}_a(s_b)_{nn} + i\sum_{m\neq n}\frac{(\partial_a H_{\mathbf{k}})_{mn}(s_b)_{nm}}{\epsilon_{n\mathbf{k}}-\epsilon_{m\mathbf{k}}} - \mathcal{A}_a(s_b)_{nn} = \mathrm{Im}\sum_{m\neq n}\frac{(\partial_a H_{\mathbf{k}})_{nm}(s_b)_{mn}}{\epsilon_{n\mathbf{k}}-\epsilon_{m\mathbf{k}}} \tag{53}$$

Comparing the above result with the gauge-invariant form of spin quadrupole moment in a periodic crystal obtained using a thermodynamic definition [2] (multiplied by a factor of $\hbar/(g\mu_B)$):

$$\begin{aligned}\mathcal{Q}_{ij} &= -\sum_{n\neq 0}\int^{\mu}\frac{d\mathbf{k}}{(2\pi)^3}(\epsilon_0+\epsilon_n-2\mu)\frac{\mathrm{Im}[(\partial_i H_{\mathbf{k}})_{0n}(s_j)_{n0}]}{(\epsilon_0-\epsilon_n)^2} \\ &= \sum_{n\neq 0}\int^{\mu}\frac{d\mathbf{k}}{(2\pi)^3}\frac{\mathrm{Im}[(\partial_i H_{\mathbf{k}})_{0n}(s_j)_{n0}]}{\epsilon_0-\epsilon_n} - 2\sum_{n\neq 0}\int^{\mu}\frac{d\mathbf{k}}{(2\pi)^3}(\epsilon_0-\mu)\frac{\mathrm{Im}[(\partial_i H_{\mathbf{k}})_{0n}(s_j)_{n0}]}{(\epsilon_0-\epsilon_n)^2}\end{aligned} \tag{54}$$

one can see that $\mathcal{M}_a^b$ corresponds to the first term, which is known to be the wave-packet contribution from the study of orbital magnetization. Our approach, however, does not work for the orbital quadrupole moment defined as [3]

$$\mathcal{M}_{ab}^o = \frac{1}{12}\langle r_a(\mathbf{r}\times\mathbf{j}-\mathbf{j}\times\mathbf{r})_b + (\mathbf{r}\times\mathbf{j}-\mathbf{j}\times\mathbf{r})_b r_a\rangle \tag{55}$$

since Eq. (17) does not hold when $[\mathbf{j},\mathbf{r}]\neq 0$.

We now proceed to the calculation of spin octupole moment using our formulas. The first term in Eq. (28) is:

$$\begin{aligned}
-\langle s_z\partial_x\partial_y\rangle &= -(s_z)_{nn}\langle u_{n\mathbf{k}}|\partial_x\partial_y|u_{n\mathbf{k}}\rangle - \sum_{m\neq n}(s_z)_{nm}\langle u_{m\mathbf{k}}|\partial_x\partial_y|u_{n\mathbf{k}}\rangle \\
&= (s_z)_{nn}(\mathcal{A}_x\mathcal{A}_y + i\partial_x\mathcal{A}_y) + (s_z)_{nn}\sum_{m\neq n}\frac{(\partial_x H_{\mathbf{k}})_{nm}(\partial_y H_{\mathbf{k}})_{mn}}{(\epsilon_{n\mathbf{k}}-\epsilon_{m\mathbf{k}})^2} \\
&+ \sum_{m\neq n}\left[-(\partial_x\partial_y H_{\mathbf{k}})_{mn} + i\mathcal{A}_y(\partial_x H_{\mathbf{k}})_{mn} + i\mathcal{A}_x(\partial_y H_{\mathbf{k}})_{mn}\right]\frac{(s_z)_{nm}}{\epsilon_{n\mathbf{k}}-\epsilon_{m\mathbf{k}}} \\
&- \sum_{l\neq n, m\neq n}\left\{\frac{(s_z)_{nm}(\partial_y H_{\mathbf{k}})_{ln}(\partial_x H_{\mathbf{k}})_{ml}}{(\epsilon_{n\mathbf{k}}-\epsilon_{l\mathbf{k}})(\epsilon_{n\mathbf{k}}-\epsilon_{m\mathbf{k}})} + (x\leftrightarrow y)\right\} \\
&+ \sum_{m\neq n}\left\{\frac{(s_z)_{nm}(\partial_y H_{\mathbf{k}})_{mn}(\partial_x H_{\mathbf{k}})_{nn}}{(\epsilon_{n\mathbf{k}}-\epsilon_{m\mathbf{k}})^2} + (x\leftrightarrow y)\right\}
\end{aligned} \tag{56}$$

One can see that the first term cancels with the first and last terms in Eq. (28) plus the intra-band contributions in the 3rd and 4th terms, while the $\mathcal{A}$ dependent terms in the 3rd term cancel with remaining inter-band contributions in the 3rd and 4th terms of Eq. (28). As a result all $\mathcal{A}$ dependent terms in Eq. (56) vanish. The final result of $\mathcal{M}_{xy}^z$ in terms of known matrix elements is

$$\begin{aligned}
\mathcal{M}_{xy}^z &= (s_z)_{nn}\sum_{m\neq n}\frac{(\partial_x H_{\mathbf{k}})_{nm}(\partial_y H_{\mathbf{k}})_{mn}}{(\epsilon_{n\mathbf{k}}-\epsilon_{m\mathbf{k}})^2} - \sum_{m\neq n}\frac{(s_z)_{nm}(\partial_x\partial_y H_{\mathbf{k}})_{mn}}{\epsilon_{n\mathbf{k}}-\epsilon_{m\mathbf{k}}} \\
&- \sum_{l\neq n, m\neq n}\left\{\frac{(s_z)_{nm}(\partial_y H_{\mathbf{k}})_{ln}(\partial_x H_{\mathbf{k}})_{ml}}{(\epsilon_{n\mathbf{k}}-\epsilon_{l\mathbf{k}})(\epsilon_{n\mathbf{k}}-\epsilon_{m\mathbf{k}})} + (x\leftrightarrow y)\right\} \\
&+ \sum_{m\neq n}\left\{\frac{(s_z)_{nm}(\partial_y H_{\mathbf{k}})_{mn}(\partial_x H_{\mathbf{k}})_{nn}}{(\epsilon_{n\mathbf{k}}-\epsilon_{m\mathbf{k}})^2} + (x\leftrightarrow y)\right\}
\end{aligned} \tag{57}$$

Recall that up to $l=3$ the wave-packet multipole moment can be made gauge invariant by replacing $\mathbf{r}$ with $\mathbf{r}-\mathbf{r}_c$. Therefore to demonstrate the true power of our general formula Eq. (27) we need to go to the $l=4$ order (hexadecapole). For definiteness we consider the $\mathcal{M}_{xyz}^a$ component ($a=x,y,z$):

$$\mathcal{M}_{xyz}^a = \frac{1}{6}\langle u_{n\mathbf{k}}|s_a(i\partial_x-\mathcal{A}_x)(i\partial_y-\mathcal{A}_y)(i\partial_z-\mathcal{A}_z)|u_{n\mathbf{k}}\rangle + (x,y,z\,\text{permutations}) \tag{58}$$

We thus first consider one term only. If $\mathcal{A}$ can be chosen to be zero at the particular $\mathbf{k}$ through a gauge transformation, we get

$$\begin{aligned}
&\langle u_{n\mathbf{k}}|s_a(i\partial_x-\mathcal{A}_x)(i\partial_y-\mathcal{A}_y)(i\partial_z-\mathcal{A}_z)|u_{n\mathbf{k}}\rangle \\
= &-i\langle s_a\partial_x\partial_y\partial_z\rangle + [\partial_x\mathcal{A}_y\langle s_a\partial_z\rangle + \partial_y\mathcal{A}_z\langle s_a\partial_x\rangle + \partial_x\mathcal{A}_z\langle s_a\partial_y\rangle] + \partial_x\partial_y\mathcal{A}_z\langle s_a\rangle
\end{aligned} \tag{59}$$

These plus their counterparts from permutation (with the 1/6 factor) give

$$\mathcal{M}_{xyz}^a = -i\langle s_a\partial_x\partial_y\partial_z\rangle + \frac{1}{2}\left[(\partial_x\mathcal{A}_y+\partial_y\mathcal{A}_x)\langle s_a\partial_z\rangle + (yz,x) + (zx,y)\right] + \frac{1}{3}[\partial_x\partial_y\mathcal{A}_z\langle s_a\rangle + (yz,x) + (zx,y)] \tag{60}$$

To go further we continue to use the gauge of $\mathcal{A}=0$, which gives

$$
\begin{aligned}
|\partial_a u_{n\mathbf{k}}\rangle &\xrightarrow{\mathcal{A}=0} \sum_{m\neq n}\frac{(\partial_a H_{\mathbf{k}})_{mn}}{\epsilon_{n\mathbf{k}}-\epsilon_{m\mathbf{k}}}|u_{m\mathbf{k}}\rangle, \qquad (61)\\
|\partial_a\partial_b u_{n\mathbf{k}}\rangle &\xrightarrow{\mathcal{A}=0} \left[-i\partial_a\mathcal{A}_b-\sum_{m\neq n}\frac{(\partial_a H_{\mathbf{k}})_{nm}(\partial_b H_{\mathbf{k}})_{mn}}{(\epsilon_{n\mathbf{k}}-\epsilon_{m\mathbf{k}})^2}\right]|u_{n\mathbf{k}}\rangle\\
&+\sum_{m\neq n}\left\{\frac{(\partial_a\partial_b H_{\mathbf{k}})_{mn}}{\epsilon_{n\mathbf{k}}-\epsilon_{m\mathbf{k}}}+\sum_{l\neq n}\frac{(\partial_b H_{\mathbf{k}})_{ln}\left[(\partial_a H_{\mathbf{k}})_{ml}-(\partial_a H_{\mathbf{k}})_{nn}\delta_{ml}\right]+(a\leftrightarrow b)}{(\epsilon_{n\mathbf{k}}-\epsilon_{l\mathbf{k}})(\epsilon_{n\mathbf{k}}-\epsilon_{m\mathbf{k}})}\right\}|u_{m\mathbf{k}}\rangle\\
|\partial_a\partial_b\partial_c u_{n\mathbf{k}}\rangle &\xrightarrow{\mathcal{A}=0} \left[-i\partial_a\partial_b\mathcal{A}_c-\sum_{m\neq n}\langle\partial_a u_{n\mathbf{k}}|u_{m\mathbf{k}}\rangle\langle u_{m\mathbf{k}}|\partial_b\partial_c u_{n\mathbf{k}}\rangle|_{\mathcal{A}=0}+(b,ca)+(ab,c)\right]|u_{n\mathbf{k}}\rangle\\
&+\sum_{m\neq n}\left\{\frac{(\partial_a\partial_b\partial_c H_{\mathbf{k}})_{mn}}{\epsilon_{n\mathbf{k}}-\epsilon_{m\mathbf{k}}}+\sum_{l\neq n}\frac{\left[(\partial_a H_{\mathbf{k}}-\partial_a\epsilon_{n\mathbf{k}})_{ml}\langle u_{l\mathbf{k}}|\partial_b\partial_c u_{n\mathbf{k}}\rangle|_{\mathcal{A}=0}+(b,ca)+(c,ab)\right]}{\epsilon_{n\mathbf{k}}-\epsilon_{m\mathbf{k}}}\right.\\
&+\left.\sum_{l\neq n}\frac{\left[((\partial_a\partial_b H_{\mathbf{k}})_{ml}-\partial_a\partial_b\epsilon_{n\mathbf{k}}\delta_{ml})(\partial_c H_{\mathbf{k}})_{ln}+(bc,a)+(ca,b)\right]}{(\epsilon_{n\mathbf{k}}-\epsilon_{m\mathbf{k}})(\epsilon_{n\mathbf{k}}-\epsilon_{l\mathbf{k}})}\right\}|u_{m\mathbf{k}}\rangle\\
&+\sum_{m\neq n}\left\{\frac{(\partial_a H_{\mathbf{k}})_{mn}}{\epsilon_{n\mathbf{k}}-\epsilon_{m\mathbf{k}}}\left[-i\partial_b\mathcal{A}_c-\sum_{l\neq n}\frac{(\partial_b H_{\mathbf{k}})_{nl}(\partial_c H_{\mathbf{k}})_{ln}}{(\epsilon_{n\mathbf{k}}-\epsilon_{l\mathbf{k}})^2}\right]+(b,ca)+(c,ab)\right\}|u_{m\mathbf{k}}\rangle
\end{aligned}
$$

Therefore only the first and last terms of $|\partial_a\partial_b\partial_c u_{n\mathbf{k}}\rangle$ contain the derivatives of $\mathcal{A}$. We focus on these terms in $-i\langle s_a\partial_x\partial_y\partial_z\rangle$ first:

$$
\begin{aligned}
&-\frac{i}{6}\left[-i\partial_x\partial_y\mathcal{A}_z\langle s_a\rangle-i\partial_y\mathcal{A}_z\langle s_a\partial_x\rangle-i\partial_z\mathcal{A}_x\langle s_a\partial_y\rangle-i\partial_x\mathcal{A}_y\langle s_a\partial_z\rangle+(x,y,z\,\text{permutations})\right] \qquad (62)\\
=&-\frac{1}{3}\left[\partial_x\partial_y A_z\langle s_a\rangle+(zx,y)+(yz,x)\right]-\frac{1}{2}\left[(\partial_x\mathcal{A}_y+\partial_y\mathcal{A}_x)\langle s_a\partial_z\rangle+(yz,x)+(zx,y)\right]
\end{aligned}
$$

which exactly cancel the last two terms in Eq. (60). Therefore the final result is

$$
\mathcal{M}^a_{xyz}=-\langle is_a\partial_x\partial_y\partial_z\rangle\Big|_{\mathcal{A}=0,\nabla\mathcal{A}\overset{!}{=}0,\nabla\nabla\mathcal{A}\overset{!}{=}0} \qquad (63)
$$

where the $\overset{!}{=}$ only means ignoring the derivatives of $\mathcal{A}$ in Eq. (61), but not in general.

## III. RASHBA SPIN-ORBIT COUPLING IN PHOSPHORENE

In this section we derive the low-energy Hamiltonian of phosphorene and most importantly the spin-orbit splitting due to a perpendicular electric field.

We start from the spin-degenerate tight-binding model of single layer phosphorene following Refs. [4, 5]. We adopt the unit cell choice depicted in Fig. 1 (a) of the main text. The four P atoms in the unit cell are located at

$$
\begin{aligned}
\mathbf{r}_A &= \mathbf{0}, \qquad (64)\\
\mathbf{r}_B &= -\delta_1\hat{x}+\frac{a_2}{2}\hat{y},\\
\mathbf{r}_C &= \frac{a_1}{2}\hat{x}+\frac{a_2}{2}\hat{y}+\delta_2\hat{z},\\
\mathbf{r}_D &= \left(\frac{a_1}{2}-\delta_1\right)\hat{x}+\delta_2\hat{z},
\end{aligned}
$$

where $a_{1,2}$ are the lattice constants along $x$ and $y$ directions, $\delta_{1,2}$ are constants that determine the puckering distortion of the phosphorene network from an ideal honeycomb lattice. The parameter values are $a_1=4.376$ Å, $a_2=3.314$ Å, $\delta_1=0.33888a_1=1.4829$ Å, $\delta_2=0.20336\times10.478=2.1308$ Å[6].

As a first approximation we only take into account spin-independent hoppings between nearest neighbors. The nearest neighbors of each site in the unit cell located at origin have the following position vectors:

$$\begin{aligned} A &: \mathbf{0}+\mathbf{r}_B,\ -\mathbf{a}_2+\mathbf{r}_B,\ \mathbf{0}+\mathbf{r}_D, \\ B &: \mathbf{0}+\mathbf{r}_A,\ \mathbf{a}_2+\mathbf{r}_A,\ -\mathbf{a}_1+\mathbf{r}_C, \\ C &: \mathbf{a}_2+\mathbf{r}_D,\ \mathbf{0}+\mathbf{r}_D,\ \mathbf{a}_1+\mathbf{r}_B, \\ D &: \mathbf{0}+\mathbf{r}_C,\ -\mathbf{a}_2+\mathbf{r}_C,\ \mathbf{0}+\mathbf{r}_A. \end{aligned} \tag{65}$$

According to [4] a low-energy tight-binding model of phosphorene can be constructed using a single orbital on each site. The model reads

$$H_0 = \sum_{\langle i\alpha, j\beta\rangle} t_{i\alpha,j\beta} c^\dagger_{i\alpha} c_{j\beta} + \text{H.c.} \tag{66}$$

where $i, j$ label unit cell and $\alpha, \beta$ label sublattices.

Due to the $D_{2h}$ symmetry we only need two nearest-neighbor hopping parameters that describe the intra- and inter-layer hoppings, respectively, which are denoted by $t_1$ and $t_2$. Ref. [4] shows that $t_1 < 0, t_2 > 0$, and $t_2 > -2t_1$. The momentum space Hamiltonian can be obtained by Fourier transform:

$$\begin{aligned} c^\dagger_{i\alpha} &= \frac{1}{N}\sum_{\mathbf{k}} e^{-i\mathbf{k}\cdot\mathbf{R}_i} c^\dagger_{\mathbf{k}\alpha} \\ &\to \frac{A_{\text{uc}}}{(2\pi)^2}\int_{\text{BZ}} d^2\mathbf{k} e^{-i\mathbf{k}\cdot\mathbf{R}_i} c^\dagger_{\mathbf{k}\alpha} \end{aligned} \tag{67}$$

which is complemented with the inverse transform

$$c^\dagger_{\mathbf{k}\alpha} = \sum_i e^{i\mathbf{k}\cdot\mathbf{R}_i} c^\dagger_{i\alpha}. \tag{68}$$

The Fourier-transformed Hamiltonian can be written as

$$H_0 = \frac{1}{N}\sum_{\mathbf{k}} C^\dagger_{\mathbf{k}} h_0(\mathbf{k}) C_{\mathbf{k}} \tag{69}$$

where $C_{\mathbf{k}} \equiv (c_{\mathbf{k}A}, c_{\mathbf{k}B}, c_{\mathbf{k}C}, c_{\mathbf{k}D})^T$. The $4\times 4$ Hermitian matrix $h_0(\mathbf{k})$ only has nonzero elements of $AB, AD, BC, CD$ in the upper triangle, which are calculated as

$$\begin{aligned} (h_0)_{AB}(\mathbf{k}) &= t_1\left(1+e^{-ia_2k_y}\right), \\ (h_0)_{AD}(\mathbf{k}) &= t_2, \\ (h_0)_{BC}(\mathbf{k}) &= t_2 e^{-ia_1k_x}, \\ (h_0)_{CD}(\mathbf{k}) &= t_1\left(1+e^{ia_2k_y}\right) \end{aligned} \tag{70}$$

Such a $h_0(\mathbf{k})$, however, is not very symmetric, which prevents us from obtaining a simple low-energy Hamiltonian. Therefore we perform the following gauge transformation by defining

$$\begin{aligned} c^\dagger_{\mathbf{k}\alpha} &= e^{i\mathbf{k}\cdot\mathbf{r}_\alpha}\sum_i e^{i\mathbf{k}\cdot\mathbf{R}_i} c^\dagger_{i\alpha} \\ c^\dagger_{i\alpha} &= \frac{1}{N}\sum_{\mathbf{k}} e^{-i\mathbf{k}\cdot(\mathbf{r}_\alpha+\mathbf{R}_i)} c^\dagger_{\mathbf{k}\alpha} \end{aligned} \tag{71}$$

As a result of this gauge transformation, we obtain

$$\begin{aligned} (h_0)_{AB}(\mathbf{k}) &= 2t_1 e^{-i\delta_1 k_x}\cos\frac{a_2k_y}{2} \\ (h_0)_{AD}(\mathbf{k}) &= t_2 e^{i\left(\frac{a_1}{2}-\delta_1\right)k_x}, \\ (h_0)_{BC}(\mathbf{k}) &= t_2 e^{-i\left(\frac{a_1}{2}-\delta_1\right)k_x} = (h_0)^*_{AD}(\mathbf{k}), \\ (h_0)_{CD}(\mathbf{k}) &= 2t_1 e^{-i\delta_1 k_x}\cos\frac{a_2k_y}{2} = (h_0)_{AB}(\mathbf{k}) \end{aligned} \tag{72}$$

and

$$h_0(\mathbf{k}) = \begin{pmatrix} h_1 & h_2 \\ h_2 & h_1 \end{pmatrix} \tag{73}$$

where

$$\begin{aligned} h_1 &= \begin{pmatrix} 0 & (h_0)_{AB}(\mathbf{k}) \\ (h_0)^*_{AB}(\mathbf{k}) & 0 \end{pmatrix}, \\ h_2 &= \begin{pmatrix} 0 & (h_0)_{AD}(\mathbf{k}) \\ (h_0)^*_{AD}(\mathbf{k}) & 0 \end{pmatrix}. \end{aligned} \tag{74}$$

$h_0(\mathbf{k})$ can therefore be block-diagonalized using

$$\begin{aligned} U^\dagger h_0(\mathbf{k}) U &= \begin{pmatrix} h_1 + h_2 & 0 \\ 0 & h_1 - h_2 \end{pmatrix} \\ &\equiv \begin{pmatrix} h_L(\mathbf{k}) & 0 \\ 0 & h_H(\mathbf{k}) \end{pmatrix}, \\ U &\equiv \frac{1}{\sqrt{2}} \begin{pmatrix} \sigma_0 & \sigma_0 \\ \sigma_0 & -\sigma_0 \end{pmatrix}. \end{aligned} \tag{75}$$

To see that $h_L$ and $h_H$ correspond to the low (closer to the band gap) and high (farther from the band gap) bands near $\Gamma$, we set $\mathbf{k} = 0$. Since

$$h_{L,H}(\mathbf{k} = 0) = (2t_1 \pm t_2)\sigma_x \tag{76}$$

have eigenvalues $\epsilon_L(\mathbf{k} = 0) = \pm|2t_1 + t_2|, \epsilon_H(\mathbf{k} = 0) = \pm|2t_1 - t_2|$ and $t_1 < 0 < t_2$, clearly $h_L$ correspond to the low-energy bands, in agreement with [5].

We next expand $h_L(\mathbf{k})$ around $\Gamma$ to get the effective continuum Hamiltonian. Note that

$$\begin{aligned} (h_0)_{AB}(\mathbf{k}) &\approx 2t_1 - 2it_1\delta_1 k_x - \frac{t_1 a_2^2}{4} k_y^2 + O(k^3), \\ (h_0)_{AD}(\mathbf{k}) &\approx t_2 + i\frac{t_2(a_1 - 2\delta_1)}{2} k_x + O(k^2). \end{aligned} \tag{77}$$

Therefore

$$\begin{aligned} h_L &\approx (2t_1 + t_2)\sigma_x \\ &- \left[-2t_1\delta_1 + \frac{t_2(a_1 - 2\delta_1)}{2}\right] k_x\sigma_y + \left(-\frac{t_1 a_2^2}{4}\right) k_y^2 \sigma_x \\ &\equiv \Delta\sigma_x - \hbar v_x k_x \sigma_y + \frac{\hbar^2}{2m_y} k_y^2 \sigma_x \end{aligned} \tag{78}$$

Using the parameter values mentioned at the beginning of this section and $t_1 = -1.486$ eV, $t_2 = 3.729$ eV [4] we can get

$$\begin{aligned} \Delta &\approx 0.757\,\mathrm{eV}, \\ \hbar v_x &\approx 7.036\,\mathrm{eV}\cdot\text{Å}, \\ \frac{\hbar^2}{2m_y} &\approx 4.08\,\mathrm{eV}\cdot\text{Å}^2 \end{aligned} \tag{79}$$

We now discuss the Rashba spin-orbit coupling induced by the perpendicular electric field. Assuming the local Wannier orbitals on each sublattice have approximate $s$-wave symmetry, a Rashba spin-orbit coupling term in the tight-binding Hamiltonian can be written as

$$H_R = \sum_{\langle i\alpha, j\beta\rangle ab} \imath\lambda^R_{i\alpha,j\beta} \left(\hat{r}_{i\alpha,j\beta} \times \mathbf{s}_{ab}\right) \cdot \hat{z} c^\dagger_{i\alpha a} c_{j\beta b} \tag{80}$$

where $a, b = \pm 1$ label spin, $\mathbf{s}$ is the spin Pauli matrix vector, and $\lambda^R_{i\alpha,j\beta}$ is the Rashba spin-orbit hopping between sites $i\alpha$ and $j\beta$ and depends on the size of the perpendicular electric field. Considering nearest neighbors only as in the spin-independent Hamiltonian, we further define $\lambda^R_{1,2}$ as the intra-plane and inter-plane nearest-neighbor Rashba spin-dependent hopping amplitudes. To Fourier transform $H_R$ we need the coefficient $\imath\lambda^R_{i\alpha,j\beta}(\hat{z}\times\hat{r}_{i\alpha,j\beta})\cdot\mathbf{s}$ for nearest neighbors, which are

$$\begin{aligned} AB &: \imath\lambda^R_1\left(-\tilde{\delta}_1 s_y \mp \frac{\tilde{a}_2}{2}s_x\right) \\ AD &: \imath\lambda^R_2 s_y \\ BC &: -\imath\lambda^R_2 s_y \\ CD &: \imath\lambda^R_1\left(-\tilde{\delta}_1 s_y \mp \frac{\tilde{a}_2}{2}s_x\right) \end{aligned} \tag{81}$$

where $\tilde{\delta}_1 \equiv \delta_1/\sqrt{\delta_1^2 + a_2^2/4}$, $\tilde{a}_2 \equiv a_2/\sqrt{\delta_1^2 + a_2^2/4}$ As a result, in the same gauge defined in Eq. (71), we have the following matrix elements in the Fourier transformed $H_R = \frac{1}{N}\sum_{\mathbf{k}} C^\dagger_{\mathbf{k}} h_R(\mathbf{k}) C_{\mathbf{k}}$:

$$\begin{aligned} (h_R)_{AB} &= -2\imath\lambda^R_1\tilde{\delta}_1 e^{-i\delta_1 k_x}\cos\frac{a_2k_y}{2}s_y + \lambda^R_1\tilde{a}_2 e^{-i\delta_1 k_x}\sin\frac{a_2k_y}{2}s_x = (h_R)_{CD} \\ (h_R)_{AD} &= \imath\lambda^R_2 e^{i\frac{a_1-2\delta_1}{2}k_x}s_y \\ (h_R)_{BC} &= -\imath\lambda^R_2 e^{-i\frac{a_1-2\delta_1}{2}k_x}s_y = [(h_R)_{AD}]^\dagger. \end{aligned} \tag{82}$$

Clearly $h_R$ has a similar structure as $h_0$. Therefore it can be block-diagonalized by the same unitary transformation:

$$U^\dagger h_R U = \begin{pmatrix} h^R_1 + h^R_2 & 0 \\ 0 & h^R_1 - h^R_2 \end{pmatrix} \tag{83}$$

where

$$\begin{aligned} h^R_1 &= \begin{pmatrix} 0 & (h_R)_{AB} \\ [(h_R)_{AB}]^\dagger & 0 \end{pmatrix}, \\ h^R_2 &= \begin{pmatrix} 0 & (h_R)_{AD} \\ [(h_R)_{AD}]^\dagger & 0 \end{pmatrix} \end{aligned} \tag{84}$$

To get the Rashba term in the low-energy continuum Hamiltonian, we expand $(h_R)_{AB}$ and $(h_R)_{AD}$ about $\Gamma$ up to first order in $k$

$$\begin{aligned} (h_R)_{AB} &\approx -2i\lambda^R_1\tilde{\delta}_1 s_y - 2\lambda^R_1\tilde{\delta}_1\delta_1 k_x s_y + \frac{\lambda^R_1\tilde{a}_2 a_2}{2}k_y s_x \\ (h_R)_{AD} &\approx i\lambda^R_2 s_y - \frac{\lambda^R_2(a_1 - 2\delta_1)}{2}k_x s_y \end{aligned} \tag{85}$$

Therefore

$$\begin{aligned} h^R_L &\equiv h^R_1 + h^R_2 \\ &\approx (2\lambda^R_1\tilde{\delta}_1 - \lambda^R_2)\sigma_y s_y - \left[2\lambda^R_1\tilde{\delta}_1\delta_1 + \frac{\lambda^R_2(a_1-2\delta_1)}{2}\right]k_x\sigma_x s_y + \frac{\lambda^R_1\tilde{a}_2 a_2}{2}k_y\sigma_x s_x \\ &\equiv \Lambda^R_0\sigma_y s_y - \Lambda^R_2 k_x\sigma_x s_y + \Lambda^R_1 k_y\sigma_x s_x \end{aligned} \tag{86}$$

Since near $\Gamma$ we expect $k_x a_1$ and $k_y a_2$ to be much smaller than 1, $k_x\Lambda^R_2$ and $k_y\Lambda^R_1$ should be much smaller than $\Lambda^R_0$. This justifies the finding in [7], namely the Rashba spin-orbit coupling near the Brillouin zone center is approximately independent of momentum and is proportional to $\sigma_y s_y$ ($\tau_y\sigma_x$ in the coordinates used in [7]).

We next look at the spin splitting of the conduction and valence bands due to $h^R_L$. This can be done by projecting $h^R_L$ into the eigenspace of $h_L$ in the spirit of degenerate perturbation theory. $h_L$ can be diagonalized by

$$\begin{aligned} U^\dagger_L h_L U_L &= \sqrt{(\Delta + \tilde{k}^2_y)^2 + \tilde{k}^2_x}\,\sigma_z, \\ U_L &= \frac{1}{\sqrt{2}}\begin{pmatrix} e^{i\phi_{\mathbf{k}}} & -e^{i\phi_{\mathbf{k}}} \\ 1 & 1 \end{pmatrix} \end{aligned} \tag{87}$$

where $\tilde{k}_y^2 \equiv \hbar^2 k_y^2/(2m_y)$, $\tilde{k}_x \equiv \hbar v_x k_x$, and $\phi_{\mathbf{k}} \equiv \arctan \frac{\tilde{k}_x}{\Delta+\tilde{k}_y^2}$. To project $h_L^R$ we only need to calculate

$$U_L^\dagger \sigma_x U_L = \cos\phi_{\mathbf{k}}\sigma_z + \sin\phi_{\mathbf{k}}\sigma_y, \qquad (88)$$
$$U_L^\dagger \sigma_y U_L = -\sin\phi\sigma_z + \cos\phi\sigma_y$$

$h_L^R$ projected to the conduction and valence bands are therefore

$$\begin{aligned} & P_c h_L^R P_c = -P_v h_L^R P_v \\ & = \Lambda_0^R s_y(-\sin\phi_{\mathbf{k}}) + (-\Lambda_2^R k_x s_y + \Lambda_1^R k_y s_x)\cos\phi_{\mathbf{k}} \\ & \approx -\left(\frac{\Lambda_0^R}{|\Delta|}\hbar v_x + \Lambda_2^R\right) k_x s_y + \Lambda_1^R k_y s_x \\ & \equiv -\alpha_x k_x s_y + \alpha_y k_y s_x \end{aligned} \qquad (89)$$

which has the form found in [8]. Since $\hbar v_x/|\Delta| \approx 10\,\text{Å}$, which is larger than the lengths $(\delta_1, a_1)$ appearing in the definition of $\Lambda_2^R$, $\alpha_x$ is likely to be dominated by $\Lambda_0^R$. This is further justified by the fact that $\alpha_x$ is one order of magnitude larger than $\alpha_y$, according to the DFT results in [8], since $\Lambda_1^R$ and $\Lambda_2^R$ should be comparable.

## IV. SYMMETRY ANALYSIS OF MULTIPOLE RESPONSES OF PHOSPHORENE

Monolayer phosphorene has $D_{2h}$ symmetry which includes the following elements:

$$E, C_2(z), C_2(y), C_2(x), i, \sigma(xy), \sigma(xz), \sigma(yz) \qquad (90)$$

with the first 5 being the generators. The perpendicular electric field breaks the $C_2(x)$, $C_2(y)$, $i$, and $\sigma(xy)$ symmetries and results in the $C_{2v}$ subgroup of $D_{2h}$, which has the following elements:

$$E, C_2(z), \sigma(xz), \sigma(yz) \qquad (91)$$

The response function for the current-induced octupole moment is a rank-4 tensor

$$\mathcal{M}_{ab}^c = \chi_{abcd} E_d. \qquad (92)$$

$\chi_{abcd}$ must be invariant under the symmetry operations in $C_{2v}$. Since the Cartesian indices $a, b, d = x, y$ correspond to polar vectors (only in-plane currents are considered here), while $c = x, y, z$ corresponds to an axial vector, they transform differently under improper rotations. Under $C_2(z)$ we have $x, y$ change sign, while $z$ is invariant, for both polar and axial indices. Since $\chi$ has four indices it is invariant under $C_2(z)$ only if there are 0, 2, or 4 indices being $z$. This excludes any components with $c = z$.

Next, for $\sigma(xz)$, $y$ is odd while $z, x$ are even for polar indices, but $y$ is even while $z, x$ are odd for axial indices. If the only axial index of $\chi$ is $y$, then the other three must be even under $\sigma(xz)$. Namely there must be 0 or 2 $y$. Conversely if the axial index of $\chi$ is $x$, the other three must include 1 or 3 $y$. Doing the same analysis for $\sigma(yz)$, we can see that if the axial index is $y$, the other three must include 0 or 2 $y$ and 1 or 3 $x$. If it is $x$, the other three must include 0 or 2 $x$ and 1 or 3 $y$. Taken together, the nonzero elements can only be

$$yyyx, xxyx, xyyy, yxyy, yyxy, yxxx, xyxx, xxxy \qquad (93)$$

For the case of $d = x$ considered in the main text, we can see that only $\mathcal{M}_{yy}^y$, $\mathcal{M}_{xx}^y$, and $\mathcal{M}_{yx}^x = \mathcal{M}_{xy}^x$ can be induced. However, $\mathcal{M}_{yy}^y$, $\mathcal{M}_{xx}^y$ are trivial since they do not correspond to staggered corner spins and only reflect the uniform spin density polarized along $y$. Similarly, when $\mathbf{E} \parallel \hat{x}$ the only nontrivial components are $\mathcal{M}_{yx}^y = \mathcal{M}_{xy}^y$.

We next discuss the nonlinear response of octupole current. For simplicity we only consider

$$\langle \mathcal{M}_{ab}^c v_x \rangle = \chi_{abcxxx}(E_x)^2. \qquad (94)$$

Again $a, b = x, y$ are polar indices while $c = x, y, z$ is axial. Following the similar steps as above one can find that only the currents of $\mathcal{M}_{yy}^y$, $\mathcal{M}_{xx}^y$, and $\mathcal{M}_{yx}^x = \mathcal{M}_{xy}^x$ are nonzero.

[1] N. Marzari, A. A. Mostofi, J. R. Yates, I. Souza, and D. Vanderbilt, Maximally localized wannier functions: Theory and applications, Rev. Mod. Phys. **84**, 1419 (2012).

[2] Y. Gao, D. Vanderbilt, and D. Xiao, Microscopic theory of spin toroidization in periodic crystals, Phys. Rev. B **97**, 134423 (2018).
[3] Y. Gao and D. Xiao, Orbital magnetic quadrupole moment and nonlinear anomalous thermoelectric transport, Phys. Rev. B **98**, 060402 (2018).
[4] A. N. Rudenko, S. Yuan, and M. I. Katsnelson, Toward a realistic description of multilayer black phosphorus: From *gw* approximation to large-scale tight-binding simulations, Phys. Rev. B **92**, 085419 (2015).
[5] D. J. P. de Sousa, L. V. de Castro, D. R. da Costa, J. M. Pereira, and T. Low, Multilayered black phosphorus: From a tight-binding to a continuum description, Phys. Rev. B **96**, 155427 (2017).
[6] S. Fukuoka, T. Taen, and T. Osada, Electronic structure and the properties of phosphorene and few-layer black phosphorus, Journal of the Physical Society of Japan **84**, 121004 (2015), https://doi.org/10.7566/JPSJ.84.121004.
[7] S. S. Baik, K. S. Kim, Y. Yi, and H. J. Choi, Emergence of Two-Dimensional Massless Dirac Fermions, Chiral Pseudospins, and Berry's Phase in Potassium Doped Few-Layer Black Phosphorus, Nano Letters **15**, 7788 (2015), pMID: 26572058, https://doi.org/10.1021/acs.nanolett.5b04106.
[8] Z. S. Popović, J. M. Kurdestany, and S. Satpathy, Electronic structure and anisotropic rashba spin-orbit coupling in monolayer black phosphorus, Phys. Rev. B **92**, 035135 (2015).
